# Supplementary material for: HARPA: A Testability-Driven, Literature-Grounded Framework for Research Ideation
Source: arXiv:2510.00620 source file (2025-10-01)
Supplement: Supplementary file 1 [file baseline.pdf]

# Paper ID

3bfb5f836d944414c171f8f843eaf90cf5604243

# Title

Adaptive Stochastic Gradient Clipping: Enhancing Stability and Convergence in Deep Learning Pipelines

# Introduction

## Problem Statement

Gradient-based optimization in deep learning often suffers from instability and slow convergence, especially in complex decision-making pipelines where gradients can become extremely large or vanishingly small. This issue can lead to poor model performance, slow training, and difficulties in fine-tuning models for specific tasks.

## Motivation

Existing methods like fixed gradient clipping, adaptive learning rates, and normalization techniques often struggle to balance stability and convergence speed across different layers and tasks within a pipeline. Inspired by the success of noise injection in improving generalization and the adaptive nature of biological neural systems, we propose a method that dynamically adjusts gradient updates based on local statistics and stochastic perturbations. This approach allows for aggressive updates in stable regions while dampening oscillations in sensitive areas, all while introducing beneficial noise for improved exploration and generalization.

# Proposed Method

We introduce Adaptive Stochastic Gradient Clipping (ASGC), which combines layer-wise gradient statistics with controlled stochastic perturbations. For each layer, we maintain running estimates of gradient mean and variance. During each update, we compute a clipping threshold as a function of these statistics. Before applying the threshold, we add Gaussian noise scaled by the layer's gradient variance. The clipping function is smoothed using a differentiable approximation, allowing end-to-end training. The noise scale and clipping function parameters are meta-learned across a diverse set of tasks.

---

# Experiments Plan

## Step-by-Step Experiment Plan

**Step 1: Implement ASGC**

Implement the ASGC algorithm as a PyTorch optimizer. This involves creating a custom optimizer class that inherits from torch.optim.Optimizer and overrides the step() method. The key components are: (1) Maintaining running estimates of gradient mean and variance for each layer. (2) Computing the adaptive clipping threshold. (3) Adding scaled Gaussian noise to the gradients. (4) Applying the smoothed clipping function. (5) Updating the parameters using the clipped and noisy gradients.

**Step 2: Prepare Datasets**

Prepare the following datasets for evaluation: (1) ImageNet for image classification. (2) WMT14 English-German for machine translation. (3) Atari suite (specifically Breakout, Pong, and Space Invaders) for reinforcement learning.

**Step 3: Setup Baseline Models**

Implement baseline models for each task: (1) ResNet-50 for ImageNet. (2) Transformer for WMT14. (3) DQN for Atari games. Train these models using standard optimizers: Adam, SGD with momentum, Adagrad, and RMSprop.

**Step 4: Train Models with ASGC**

Train the same model architectures using ASGC. Use a grid search to find optimal hyperparameters for ASGC, including the initial noise scale and clipping function parameters.

**Step 5: Evaluate Performance**

Compare ASGC against baselines on the following metrics: (1) Final test accuracy/BLEU score/game score. (2) Training time to reach a specific performance threshold. (3) Stability of training (measured by the variance of validation performance across epochs). (4) Generalization (measured by the gap between training and test performance).

**Step 6: Analyze Robustness**

Evaluate the robustness of ASGC to hyperparameter choices by training models with randomly sampled hyperparameters and comparing the distribution of final performances against baselines.

**Step 7: Visualize Gradient Statistics**

Plot the distribution of gradient magnitudes before and after clipping for different layers and at different stages of training. Compare these distributions between ASGC and baseline optimizers.

**Step 8: Analyze Meta-Learned Parameters**

Examine the learned noise scales and clipping function parameters across different tasks and model architectures. Visualize how these parameters evolve during training.

**Step 9: Ablation Studies**

Conduct ablation studies to isolate the effects of adaptive clipping and stochastic perturbations. Train models with only adaptive clipping (no noise) and only stochastic perturbations (fixed clipping threshold).

**Step 10: Write Up Results**

Compile all results, visualizations, and analyses into a comprehensive report or paper draft.

## Test Case Examples

### Baseline Prompt Input

Train a ResNet-50 model on ImageNet using Adam optimizer with default hyperparameters.

### Baseline Prompt Expected Output

Final Top-1 Accuracy: 76.1%, Training Time: 90 hours, Stability (std dev of validation accuracy over last 10 epochs): 0.5%

### Proposed Prompt Input

Train a ResNet-50 model on ImageNet using ASGC optimizer with meta-learned hyperparameters.

### Proposed Prompt Expected Output

Final Top-1 Accuracy: 77.3%, Training Time: 85 hours, Stability (std dev of validation accuracy over last 10 epochs): 0.3%

### Explanation

ASGC achieves higher accuracy in less training time, with improved stability during the final stages of training. This demonstrates the benefits of adaptive clipping and stochastic perturbations in balancing aggressive updates and stability.

## Fallback Plan

If ASGC does not outperform baselines as expected, we can pivot the project to an in-depth analysis of why adaptive stochastic methods struggle in certain scenarios. We would conduct a series of experiments to isolate the effects of gradient clipping, noise injection, and adaptive thresholds on different types of neural architectures and tasks. This could involve visualizing gradient flow through networks, analyzing the spectrum of the Hessian at different stages of training, and studying how different optimization techniques affect the loss landscape. We could also explore combining ASGC with other advanced optimization techniques like layer-wise adaptive rates or Hessian-based preconditioning. The goal would be to provide insights into the interplay between network architecture, task complexity, and optimization dynamics, potentially informing the development of next-generation optimization algorithms.

## References


1. The Limited Multi-Label Projection Layer (2019)
2. Optimizing Rank-Based Metrics With Blackbox Differentiation (2019)
3. Categorical Reparameterization with Gumbel-Softmax (2016)
4. Differentiable Top-k Operator with Optimal Transport (2020)
5. Tackling Prevalent Conditions in Unsupervised Combinatorial Optimization: Cardinality, Minimum, Covering, and More (2024)
6. Differentiable Combinatorial Scheduling at Scale (2024)
7. Fast Differentiable Sorting and Ranking (2020)
8. Differentiation of Blackbox Combinatorial Solvers (2019)
9. Deep Network Flow for Multi-object Tracking (2017)
10. Learning Latent Trees with Stochastic Perturbations and Differentiable Dynamic Programming (2019)
