# Supplementary material for: HARPA: A Testability-Driven, Literature-Grounded Framework for Research Ideation
Source: arXiv:2510.00620 source file (2025-10-01)
Supplement: Supplementary file 2 [file harpa_example.pdf]

# Paper ID

3bfb5f836d944414c171f8f843eaf90cf5604243

# Title

Combining stochastic softmax tricks with control variates for improved spanning tree optimization.

# Introduction

## Problem Statement

Integrating stochastic softmax tricks with control variates will significantly improve convergence speed and stability in spanning tree optimization problems compared to using stochastic softmax tricks alone.

## Motivation

Existing methods for variance reduction in discrete optimization problems often focus on individual techniques like Rao-Blackwellization or stochastic softmax tricks in isolation. However, these approaches do not fully exploit the potential synergies between different variance reduction techniques, particularly in complex combinatorial spaces like spanning trees and arborescences. No prior work has explored the integration of stochastic softmax tricks with control variates specifically for spanning tree problems, which could offer significant improvements in convergence speed and stability by leveraging structured relaxations and variance reduction simultaneously.

# Proposed Method

The research aims to explore the integration of stochastic softmax tricks with control variates to enhance variance reduction in spanning tree optimization problems. Stochastic softmax tricks provide structured relaxations that allow for gradient estimation in combinatorial spaces, while control variates reduce the variance of these gradient estimators by incorporating additional information. By combining these two techniques, the hypothesis posits that the model will achieve faster convergence and more stable performance. This approach addresses the gap in existing research where these techniques are typically applied in isolation. The expected outcome is a more efficient optimization process, particularly in graph-based problems like spanning trees, where maintaining the graph structure is crucial for accurate gradient computation. This combination is expected to reduce the variance of gradient estimates more effectively than either technique alone, leading to improved model performance metrics such as convergence speed and stability.

## Background

Stochastic Softmax Tricks: Stochastic softmax tricks are used to create structured relaxations for combinatorial optimization problems, such as spanning trees. This involves using the Gumbel-Max trick to reparameterize distributions over one-hot binary vectors, allowing for gradient estimation in discrete distributions. The structured relaxation maintains the graph structure, enabling efficient gradient computation. This technique was selected for its ability to handle complex combinatorial spaces and its compatibility with gradient-based optimization methods.

Control Variates: Control variates are used to reduce the variance of gradient estimators by incorporating additional information into the estimation process. This involves constructing a control variate based on an analytical linear approximation to the gradient estimator, which is then combined with a naïve gradient estimate. This method remains unbiased while achieving lower variance, particularly effective in Gaussian approximating families. The control variate is expected to enhance the efficiency of the stochastic softmax tricks by further reducing the variance of the gradient estimates.

## Implementation

The proposed method involves integrating stochastic softmax tricks with control variates to optimize spanning tree problems. First, the stochastic softmax tricks are applied to

create a structured relaxation of the spanning tree problem, allowing for gradient estimation in a differentiable manner. This is achieved by representing the problem as a linear program and applying a softmax function to approximate the selection of edges. Next, control variates are introduced to further reduce the variance of the gradient estimators. This involves constructing a control variate based on an analytical linear approximation to the gradient estimator, which is then combined with the gradient estimates obtained from the stochastic softmax tricks. The integration occurs at the gradient computation stage, where the control variate is used to adjust the gradient estimates, leading to lower variance and improved convergence. The data flows from the structured relaxation to the control variate adjustment, with the final output being a more stable and efficient gradient estimate. This method is implemented using libraries that support automatic differentiation, such as TensorFlow or PyTorch, and is evaluated against baseline methods like the vanilla Gumbel-Softmax estimator.

---

# Experiments Plan

## Operationalization Information

Please implement an experiment to test the hypothesis that integrating stochastic softmax tricks with control variates will significantly improve convergence speed and stability in spanning tree optimization problems compared to using stochastic softmax tricks alone.

**Experiment Overview**

This experiment will compare three methods for spanning tree optimization:
1. **Baseline 1**: Vanilla Gumbel-Softmax estimator
2. **Baseline 2**: Stochastic softmax tricks without control variates
3. **Experimental**: Stochastic softmax tricks integrated with control variates

**2. Stochastic Softmax Tricks without Control Variates (Baseline 2)**

Implement structured relaxations for spanning trees:
- Represent the spanning tree polytope using the cycle constraints
- Apply stochastic softmax tricks to maintain the graph structure
- Use automatic differentiation to compute gradients
- Implement a projection step to ensure the solution is a valid spanning tree

**3. Integrated Approach with Control Variates (Experimental)**

The experiment should measure convergence speed (iterations to reach a predefined accuracy threshold) and stability (variance of predictions across different runs) for each method.

**Implementation Details**

**Pilot Mode Settings**

Implement a global variable `PILOT_MODE` with three possible settings: `MINI_PILOT`, `PILOT`, or `FULL_EXPERIMENT`.
- **MINI_PILOT**: Use 5 small random graphs (10-15 nodes) and run 10 optimization iterations with 3 independent runs per method
- **PILOT**: Use 20 medium-sized random graphs (20-50 nodes) and run 50 optimization iterations with 10 independent runs per method
- **FULL_EXPERIMENT**: Use 100 graphs of varying sizes (up to 100 nodes) and run 200 optimization iterations with 30 independent runs per method

The experiment should first run in MINI_PILOT mode, then PILOT mode if successful, but stop before FULL_EXPERIMENT (which will be manually triggered after human verification).

**Graph Dataset Generation**

Use NetworkX to generate the following types of random graphs for the experiment:
1. Erdős–Rényi random graphs

Extend the stochastic softmax tricks implementation with control variates:
- Construct a control variate based on an analytical linear approximation to the gradient estimator
- Combine the control variate with the naïve gradient estimate from the stochastic softmax tricks
- Implement the optimal scaling parameter for the control variate
- Apply the adjusted gradient in the optimization process

**Optimization Task**

Implement a minimum spanning tree optimization task where the objective is to find the spanning tree with minimum total edge weight. Additionally, implement a maximum spanning tree task as a secondary objective.

**Evaluation Metrics**

1. **Convergence Speed**: Measure the number of iterations required to reach 95% of the optimal solution
2. **Stability**: Calculate the variance of the solutions across multiple independent runs
3. **Solution Quality**: Compare the final solution to the true optimal spanning tree (computed using standard MST algorithms)
4. **Gradient Variance**: Measure the variance of the gradient estimates during optimization

**Experiment Procedure**

2. Barabási–Albert preferential attachment graphs
3. Watts–Strogatz small-world graphs

For each graph, assign random edge weights from a uniform distribution [0.1, 10.0].

**Method Implementations**

**1. Vanilla Gumbel-Softmax Estimator (Baseline 1)**

Implement the standard Gumbel-Softmax trick for spanning tree optimization:
- Represent the graph as an edge selection problem
- Apply the Gumbel-Max trick to sample spanning trees
- Use the softmax temperature parameter to control the discreteness of the distribution
- Implement straight-through estimation for the backward pass

1. For each graph in the dataset:
   a. Run each method (Baseline 1, Baseline 2, Experimental) multiple times with different random seeds
   b. Record the optimization trajectory (objective value vs. iteration)
   c. Measure the gradient variance at each iteration
   d. Calculate the final solution quality

1. Aggregate results across all graphs and runs:
   a. Calculate average convergence speed for each method
   b. Calculate average stability for each method
   c. Perform statistical significance tests (bootstrap resampling) to compare methods

**Visualization and Reporting**

1. Generate convergence plots showing objective value vs. iteration for each method
2. Create box plots showing the distribution of convergence speeds and stability metrics
3. Generate tables with summary statistics for each method
4. Visualize example spanning trees produced by each method on selected graphs

**Implementation Notes**

- Use PyTorch for automatic differentiation and gradient computation
- Use NetworkX for graph manipulation and visualization
- Implement proper seeding for reproducibility
- Use a learning rate scheduler to improve convergence
- Save intermediate results to allow for experiment resumption

**Expected Output**

The experiment should produce:
1. A comprehensive report comparing the three methods
2. Convergence plots for each method
3. Statistical analysis of the differences between methods
4. Visualizations of example spanning trees
5. Raw data for further analysis

Please implement this experiment and run it first in MINI_PILOT mode, then in PILOT mode if successful. Do not proceed to FULL_EXPERIMENT mode without human verification.

*End Note:*

*The source paper is Paper 0: Learning with Differentiable Perturbed Optimizers (109 citations, 2020). This idea draws upon a trajectory of prior work, as seen in the following sequence: Paper 1 --> Paper 2 --> Paper 3 --> Paper 4 --> Paper 5. The analysis reveals a consistent theme of addressing the high variance in gradient estimation for discrete latent variables, a challenge initially highlighted in the source paper. The*

*progression of research has introduced various techniques like stochastic softmax tricks, Rao-Blackwellization, and coupled gradient estimators to tackle this issue. However, these approaches often focus on specific applications or settings, such as combinatorial spaces or categorical variables. A novel research idea could involve developing a generalized framework that unifies these variance reduction techniques, making them adaptable to a broader range of discrete optimization problems. This would advance the field by providing a more versatile tool for training models with discrete components, addressing the limitations of existing methods that are often application-specific.*

*The initial trend observed from the progression of related work highlights a consistent research focus. However, the final hypothesis proposed here is not merely a continuation of that trend — it is the result of a deeper analysis of the hypothesis space. By identifying underlying gaps and reasoning through the connections between works, the idea builds on, but meaningfully diverges from, prior directions to address a more specific challenge.*

---

## References


1. Learning with Differentiable Perturbed Optimizers (2020)
2. Gradient Estimation with Stochastic Softmax Tricks (2020)
3. Rao-Blackwellizing the Straight-Through Gumbel-Softmax Gradient Estimator (2020)
4. Coupled Gradient Estimators for Discrete Latent Variables (2021)
5. Training Discrete Deep Generative Models via Gapped Straight-Through Estimator (2022)
6. Revisiting the Gumbel-Softmax in MADDPG (2023)
7. Rao-Blackwellized Stochastic Gradients for Discrete Distributions (2018)
8. Tackling Data Heterogeneity: A New Unified Framework for Decentralized SGD with Sample-induced Topology (2022)
9. A generalized approximate control variate framework for multifidelity uncertainty quantification (2018)
10. Adaptive Variance Reduction for Stochastic Optimization under Weaker Assumptions (2024)
11. On Variance Reduction in Stochastic Gradient Descent and its Asynchronous Variants (2015)

12. Partial Variance Reduction improves Non-Convex Federated learning on heterogeneous data (2022)
13. Improved Analysis and Rates for Variance Reduction under Without-replacement Sampling Orders (2021)
14. Stochastic Variance Reduction Methods for Policy Evaluation (2017)
15. Reducing Reparameterization Gradient Variance (2017)
